# Supplementary material for: The role of electron localization in density functionals
Source: arXiv:1409.5666 source file (2014-09-19)
Supplement: Supplementary file 1 [file Supplemental_Material.pdf]

# The role of electron localization in density functionals (supplemental material)

M. J. P. Hodgson, J. D. Ramsden, T. R. Durrant, and R. W. Godby
*Department of Physics, University of York and European Theoretical Spectroscopy Facility, Heslington, York YO10 5DD, United Kingdom*
(Dated: June 13, 2014)

## SYSTEM 1 (DOUBLE WELL)

The external potential is (we use Hartree atomic units)

$$V_{\text{ext}} = -\frac{1}{4}\left[e^{-\frac{1}{100}(x-20)^2} + e^{-\frac{1}{100}(x+20)^2}\right] + \frac{3}{20}\theta(x-10), \tag{1}$$

where $\theta(x)$ is the Heaviside step function. For this system converged results are obtained with $\delta x = 0.16$ a.u. Figure 1 shows the external potential with the ground-state density.

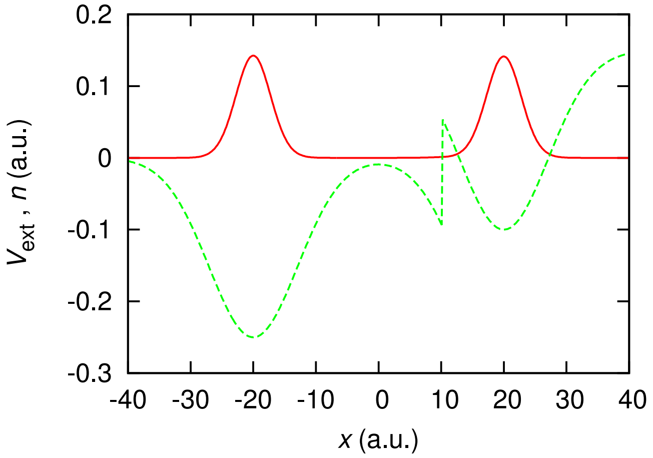


FIG. 1: *System 1.* The external potential (dashed green) with the ground-state density (solid red).

## SYSTEM 2 (SINGLE WELL)

The external potential is

$$V_{\text{ext}} = -e^{-\frac{x^2}{10}}, \tag{2}$$

with a grid spacing $\delta x = 0.028$ a.u. Figure 2 shows the external potential with the ground-state density.

## SYSTEM 3 (POLARIZED THREE-ATOM CHAIN)

The external potential is

$$V_{\text{ext}} = -\frac{1}{2}\left[e^{-\frac{1}{10}(x-15)^2} + e^{-\frac{1}{10}x^2} + e^{-\frac{1}{10}(x+15)^2}\right] - \frac{x}{100}, \tag{3}$$

with a grid spacing $\delta x = 0.2$ a.u. Figure 3 shows the external potential with the ground-state density.

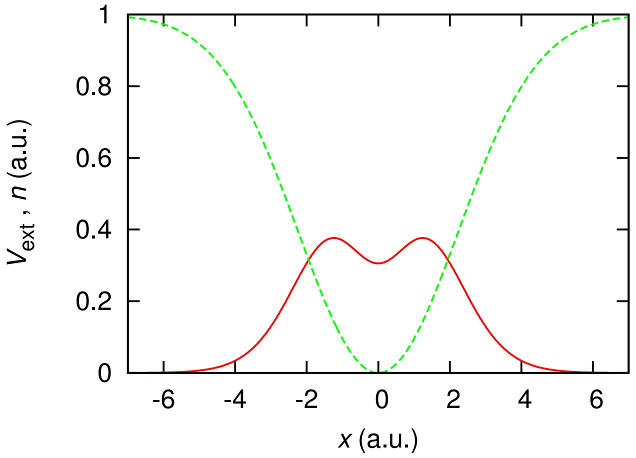


FIG. 2: *System 2.* The external potential (dashed green) with the ground-state density (solid red).

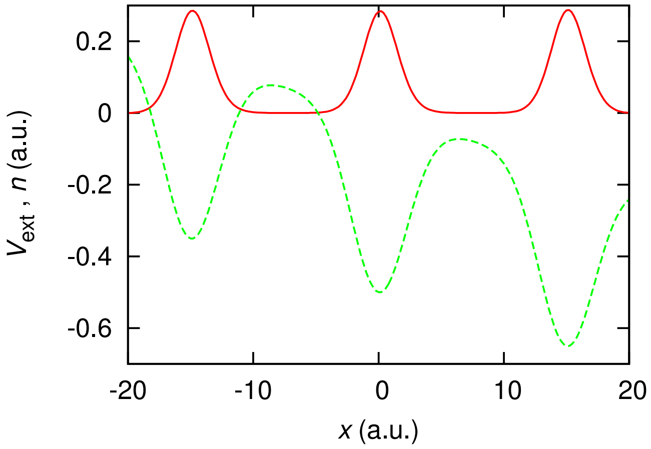


FIG. 3: *System 3.* The external potential (dashed green) with the ground-state density (solid red).

## SYSTEM 4 (TIME-DEPENDENT DOUBLE WELL)

The external potential for the ground-state system is

$$V_{\rm ext} = -\frac{1}{2}\left[e^{-\frac{1}{4}(x-5)^2} + e^{-\frac{1}{4}(x+5)^2}\right] \tag{4}$$

with grid spacing $\delta x = 0.04$ a.u. and time step $\delta t = 5\times10^{-4}$ a.u. For $t \geq 0$ an additional electric field ($\Delta V_{\rm ext} = -0.1x$) is applied. Figure 4(a) shows the ground-state external potential and the time-dependent potential. Figure 4(b) shows the ground-state electron density and the electron density at $t = 5$ a.u.

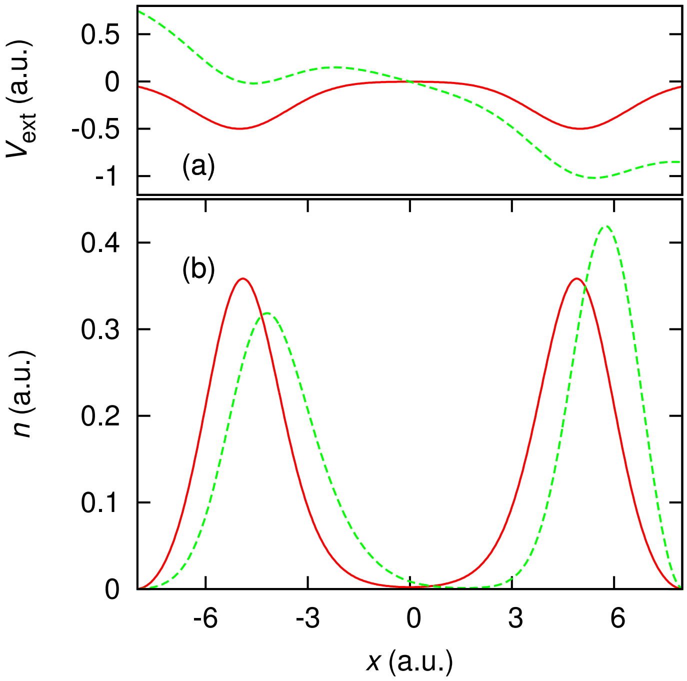


FIG. 4: *System 4*. (a) The external potential for the ground state (solid red) and the external potential for $t \geq 0$ (dashed green). (b) The ground-state electron density (solid red) and the electron density at $t = 5$ a.u.
